# Supplementary material for: ETAP: Energy-aware Timing Analysis of Intermittent Programs
Source: arXiv:2201.11433 source file (2022-02-03)
Supplement: Supplementary file 1 [file appendix.tex]

% \newpage
%\input{related_tab}
